# Supplementary material for: CLIP2StyleGAN: Unsupervised Extraction of StyleGAN Edit Directions
Source: arXiv:2112.05219 source file (2021-12-09)
Supplement: Supplementary file 1 [file supplementary_table1.tex]

\centering
\scriptsize
\begin{center}

\begin{tabular}{rrrr} \toprule

 \multicolumn{1}{c}{Attribute}   & \multicolumn{1}{c}{P_A \uparrow} & \multicolumn{1}{c}{P_B \uparrow} & \multicolumn{1}{c}{N_A \downarrow}  \\ \midrule

Asian  &\{Asian\} &\{Korean\} \hspace{0.2cm} &\{Non-Asian\}\hspace{0.1cm}		 \\  
\midrule
CLIP  &0.4412	&0.3228 \hspace{0.3cm} &0.2361 \hspace{0.4cm}	  	 \\  
SG-ours  &0.4990	&0.1185  \hspace{0.3cm} &0.3826	\hspace{0.4cm} \\  
\midrule

Glass  &\{Glass\} &\{Specs\} \hspace{0.2cm} &\{No glass\}	\hspace{0.2cm} \\
\midrule
CLIP  &0.8729	&0.1042 \hspace{0.3cm} &0.0236   \hspace{0.4cm}	 \\
SG  &0.7772	&0.1483 \hspace{0.3cm}  &0.0746	\hspace{0.4cm} \\
\midrule

Black  &\{Black\} &\{African\}  \hspace{0.2cm} &\{Non-Black\} \hspace{0.1cm}	 \\
\midrule
CLIP  &0.6157	&0.2488 \hspace{0.3cm} &0.1353   \hspace{0.4cm}	 \\
SG  &0.5181	&0.3242 \hspace{0.3cm} &0.1580	\hspace{0.4cm} \\

\bottomrule
\end{tabular}
\end{center}

\centering
\scriptsize
\begin{center}
    
\def\ua{\ensuremath{\uparrow}}
\def\da{\ensuremath{\downarrow}}

\begin{tabular}{rccc} \toprule

 \multicolumn{1}{c}{Image-Sets}   & 
 %\multicolumn{1}{c}{P_A \uparrow} & \multicolumn{1}{c}{P_B \uparrow} & \multicolumn{1}{c}{N_A \downarrow} 
  \multicolumn{3}{c}{CLIP ZS Classifier Score}
 \\ %\midrule

  & Kids\ua & Teens\ua & Adults\da 	 \\  
%\midrule
CLIP($\mathcal{X}^+$)  &0.8462 &0.1257 &0.0281  	 \\  
SG-ours  &\textbf{0.8252}	&0.1266  &\textbf{0.0480} 		 \\  
GANSpace  &0.3442	&\textbf{0.4932}  &0.1626 		 \\  
\midrule
  &Beard\ua &\ Facial-Hair\ua & Clean-Shaved\da	 \\
%\midrule
CLIP($\mathcal{X}^+$)  &0.8052 &0.1913 &0.0033   \\
SG-ours  &0.5486	&\textbf{0.4465} &\textbf{0.0146}\\
GANSpace  &\textbf{0.6328}	&0.3284 &0.0386	 \\
\midrule

  &Smile\ua & Happy\ua &Sad\da \\
%\midrule
CLIP($\mathcal{X}^+$)  &\textit{0.9170}	&\textit{0.0814}  &\textit{0.0019}  	 \\
SG-ours  &\textbf{0.9092}	&\textbf{0.0859}  &\textbf{0.0047} 	 \\
GANSpace  &0.9082	&0.0858  &0.0059	 \\
\midrule
 &Male\ua & Masculine\ua  &Female\da  \\
%\midrule
CLIP($\mathcal{X}^+$)  &0.7139	&0.2751 &0.0108  	 \\
SG-ours  &\textbf{0.6914}	&0.2837 &\textbf{0.0248} \\
GANSpace  &0.5811	&\textbf{0.3870}  &0.0323\\

\bottomrule
\end{tabular}
\end{center}
